# Supplementary material for: DL-IAPS and PJSO: A Path/Speed Decoupled Trajectory Optimization and its Application in Autonomous Driving
Source: arXiv:2009.11135 source file (2020-09-23)
Supplement: Supplementary file 1 [file appendix.tex]

%auto-ignore
